# Supplementary material for: Kernel-based multi-step predictors for data-driven analysis and control of nonlinear systems through the velocity form
Source: arXiv:2408.00688 source file (2024-08-01)
Supplement: Supplementary file 1 [file appendix.tex]

\appendices
\section{Regressor form with larger lag}\label{app:regressoradd}
\begingroup\allowdisplaybreaks
Let us now consider a system with a larger lag:
\begin{multline}
    y(k) = a_{10}y(k-1) + a_{11} p(k-1) y(k-1) + a_{20}y(k-2) + a_{21} p(k-2) y(k-2) \\ + b_{10}u(k-1) + b_{11} p(k-1) u(k-1) + b_{20}u(k-2) + b_{21} p(k-2) u(k-2).
\end{multline}
That is:
\begin{align}
    y(k) & = \underbrace{\begin{bmatrix} a_{10} & a_{11} & a_{20} & a_{21} & b_{10} & b_{11} & b_{20} & b_{21} \end{bmatrix}}_{\theta_0}\underbrace{\begin{bmatrix}
        y(k-1)\\p(k-1) y(k-1)\\y(k-2)\\p(k-2) y(k-2) \\u(k-1) \\p(k-1) u(k-1)\\u(k-2) \\ p(k-2) u(k-2)
    \end{bmatrix}}_{\varphi_0}\\
    y(k+1) & = a_{10}\theta_0\varphi_0 + a_{11}p(k)\theta_0\varphi_0 +\begin{bmatrix}  a_{20} & a_{21} & b_{10} & b_{11} & b_{20} & b_{21} \end{bmatrix}\begin{bmatrix}
        y(k-1)\\p(k-1) y(k-1) \\u(k) \\p(k) u(k)\\u(k-1) \\ p(k-1) u(k-1)
    \end{bmatrix} \\
    &\quad \text{ Let: }\hat{\theta}_1 := \begin{bmatrix} a_{20} & a_{21} &0&0& b_{20} & b_{21}&0&0 \end{bmatrix}, \text{ such that:} \\
    & = (a_{10}\theta_0 + \hat{\theta}_1)\varphi_0 + a_{11}\theta_0p(k)\varphi_0 + \begin{bmatrix} b_{10} & b_{11} \end{bmatrix}\begin{bmatrix} u(k) \\p(k) u(k) \end{bmatrix} \\
    & = \underbrace{\begin{bmatrix} (a_{10}\theta_0 + \hat{\theta}_1) & a_{11}\theta_0 & b_{10} & b_{11} \end{bmatrix}}_{\theta_1} \begin{bmatrix}\varphi_0 \\p(k) \varphi_0\\u(k) \\p(k) u(k) \end{bmatrix} = \theta_1\underbrace{\begin{bmatrix}\begin{bsmallmatrix} 1 \\ p(k) \end{bsmallmatrix}\kron I_{n_\varphi} & 0 \\ 0 & \begin{bsmallmatrix} 1 \\ p(k) \end{bsmallmatrix}\kron I_{\dnu}\end{bmatrix}}_{\mt{P}_1}\begin{bmatrix}\varphi_0\\u(k)\end{bmatrix}\\
    y(k+2) & = \begin{bmatrix} a_{10} & a_{11} & a_{20} & a_{21} & b_{10} & b_{11} & b_{20} & b_{21} \end{bmatrix}\begin{bmatrix} y(k+1)\\p(k+1) y(k+1)\\y(k)\\p(k) y(k) \\u(k+1) \\p(k+1) u(k+1)\\u(k) \\ p(k) u(k)\end{bmatrix}\\
        & = a_{10}\theta_1\mt{P}_1\begin{bmatrix} \varphi_0\\u(k) \end{bmatrix} + a_{11}p(k+1)\theta_1\mt{P}_1\begin{bmatrix} \varphi_0\\u(k) \end{bmatrix} + a_{20}\theta_0\varphi_0 + a_{21}p(k)\theta_0\varphi_0 + \begin{bmatrix} b_{10} & b_{11} & b_{20} & b_{21} \end{bmatrix} \begin{bmatrix} u(k+1) \\p(k+1) u(k+1)\\u(k) \\ p(k) u(k)\end{bmatrix} \\
        & = a_{10}\theta_1\mt{P}_1\begin{bmatrix} \varphi_0\\u(k) \end{bmatrix} + a_{11}\theta_1p(k+1)\mt{P}_1\begin{bmatrix} \varphi_0\\u(k) \end{bmatrix} + a_{20}\theta_0\varphi_0 + a_{21}\theta_0p(k)\varphi_0 + \begin{bmatrix} b_{10} & b_{11} & b_{20} & b_{21} \end{bmatrix} \begin{bmatrix} u(k+1) \\p(k+1) u(k+1)\\u(k) \\ p(k) u(k)\end{bmatrix} \\
        & = a_{10}\theta_1\mt{P}_1\begin{bmatrix} \varphi_0\\u(k) \end{bmatrix} + a_{11}\theta_1p(k+1)\mt{P}_1\begin{bmatrix} \varphi_0\\u(k) \end{bmatrix} + \underbrace{\begin{bmatrix}a_{20}\theta_0& a_{21}\theta_0 & b_{20} & b_{21} \end{bmatrix}}_{\hat{\theta}_2} \underbrace{\begin{bmatrix}\varphi_0 \\p(k) \varphi_0\\u(k) \\p(k) u(k) \end{bmatrix}}_{\mt{P}_1\begin{bmatrix} \varphi_0\\u(k) \end{bmatrix}} +  \begin{bmatrix} b_{10} & b_{11}  \end{bmatrix} \begin{bmatrix} u(k+1) \\p(k+1) u(k+1)\end{bmatrix} \\
        & = \begin{bmatrix} \begin{bmatrix} a_{10}\theta_1+\hat{\theta}_2 & a_{11}\theta_1\end{bmatrix} & \begin{bmatrix} b_{10} & b_{11} \end{bmatrix}  \end{bmatrix} \begin{bmatrix} \begin{bsmallmatrix} 1\\p(k+1) \end{bsmallmatrix}\kron I_{(1+\dnp)(n_\varphi+\dnu)} & 0 \\ 0 & \begin{bsmallmatrix} 1\\p(k+1) \end{bsmallmatrix}\kron I_{\dnu} \end{bmatrix}\begin{bmatrix} \mt{P}_1 & 0 \\ 0 & I_{\dnu}\end{bmatrix}\begin{bmatrix} \varphi_0\\u(k) \\ u(k+1)\end{bmatrix}
\end{align}
\endgroup
